# Supplementary material for: Visual Writing Prompts: Character-Grounded Story Generation with Curated Image Sequences
Source: arXiv:2301.08571 source file (2023-01-20)
Supplement: Supplementary file 1 [file appendix.tex]

% XH: temporary; need a seperate document

% \begin{figure*}[ht]
% \includegraphics[width=0.96\textwidth,trim={0cm 16cm 0cm 1cm},clip]{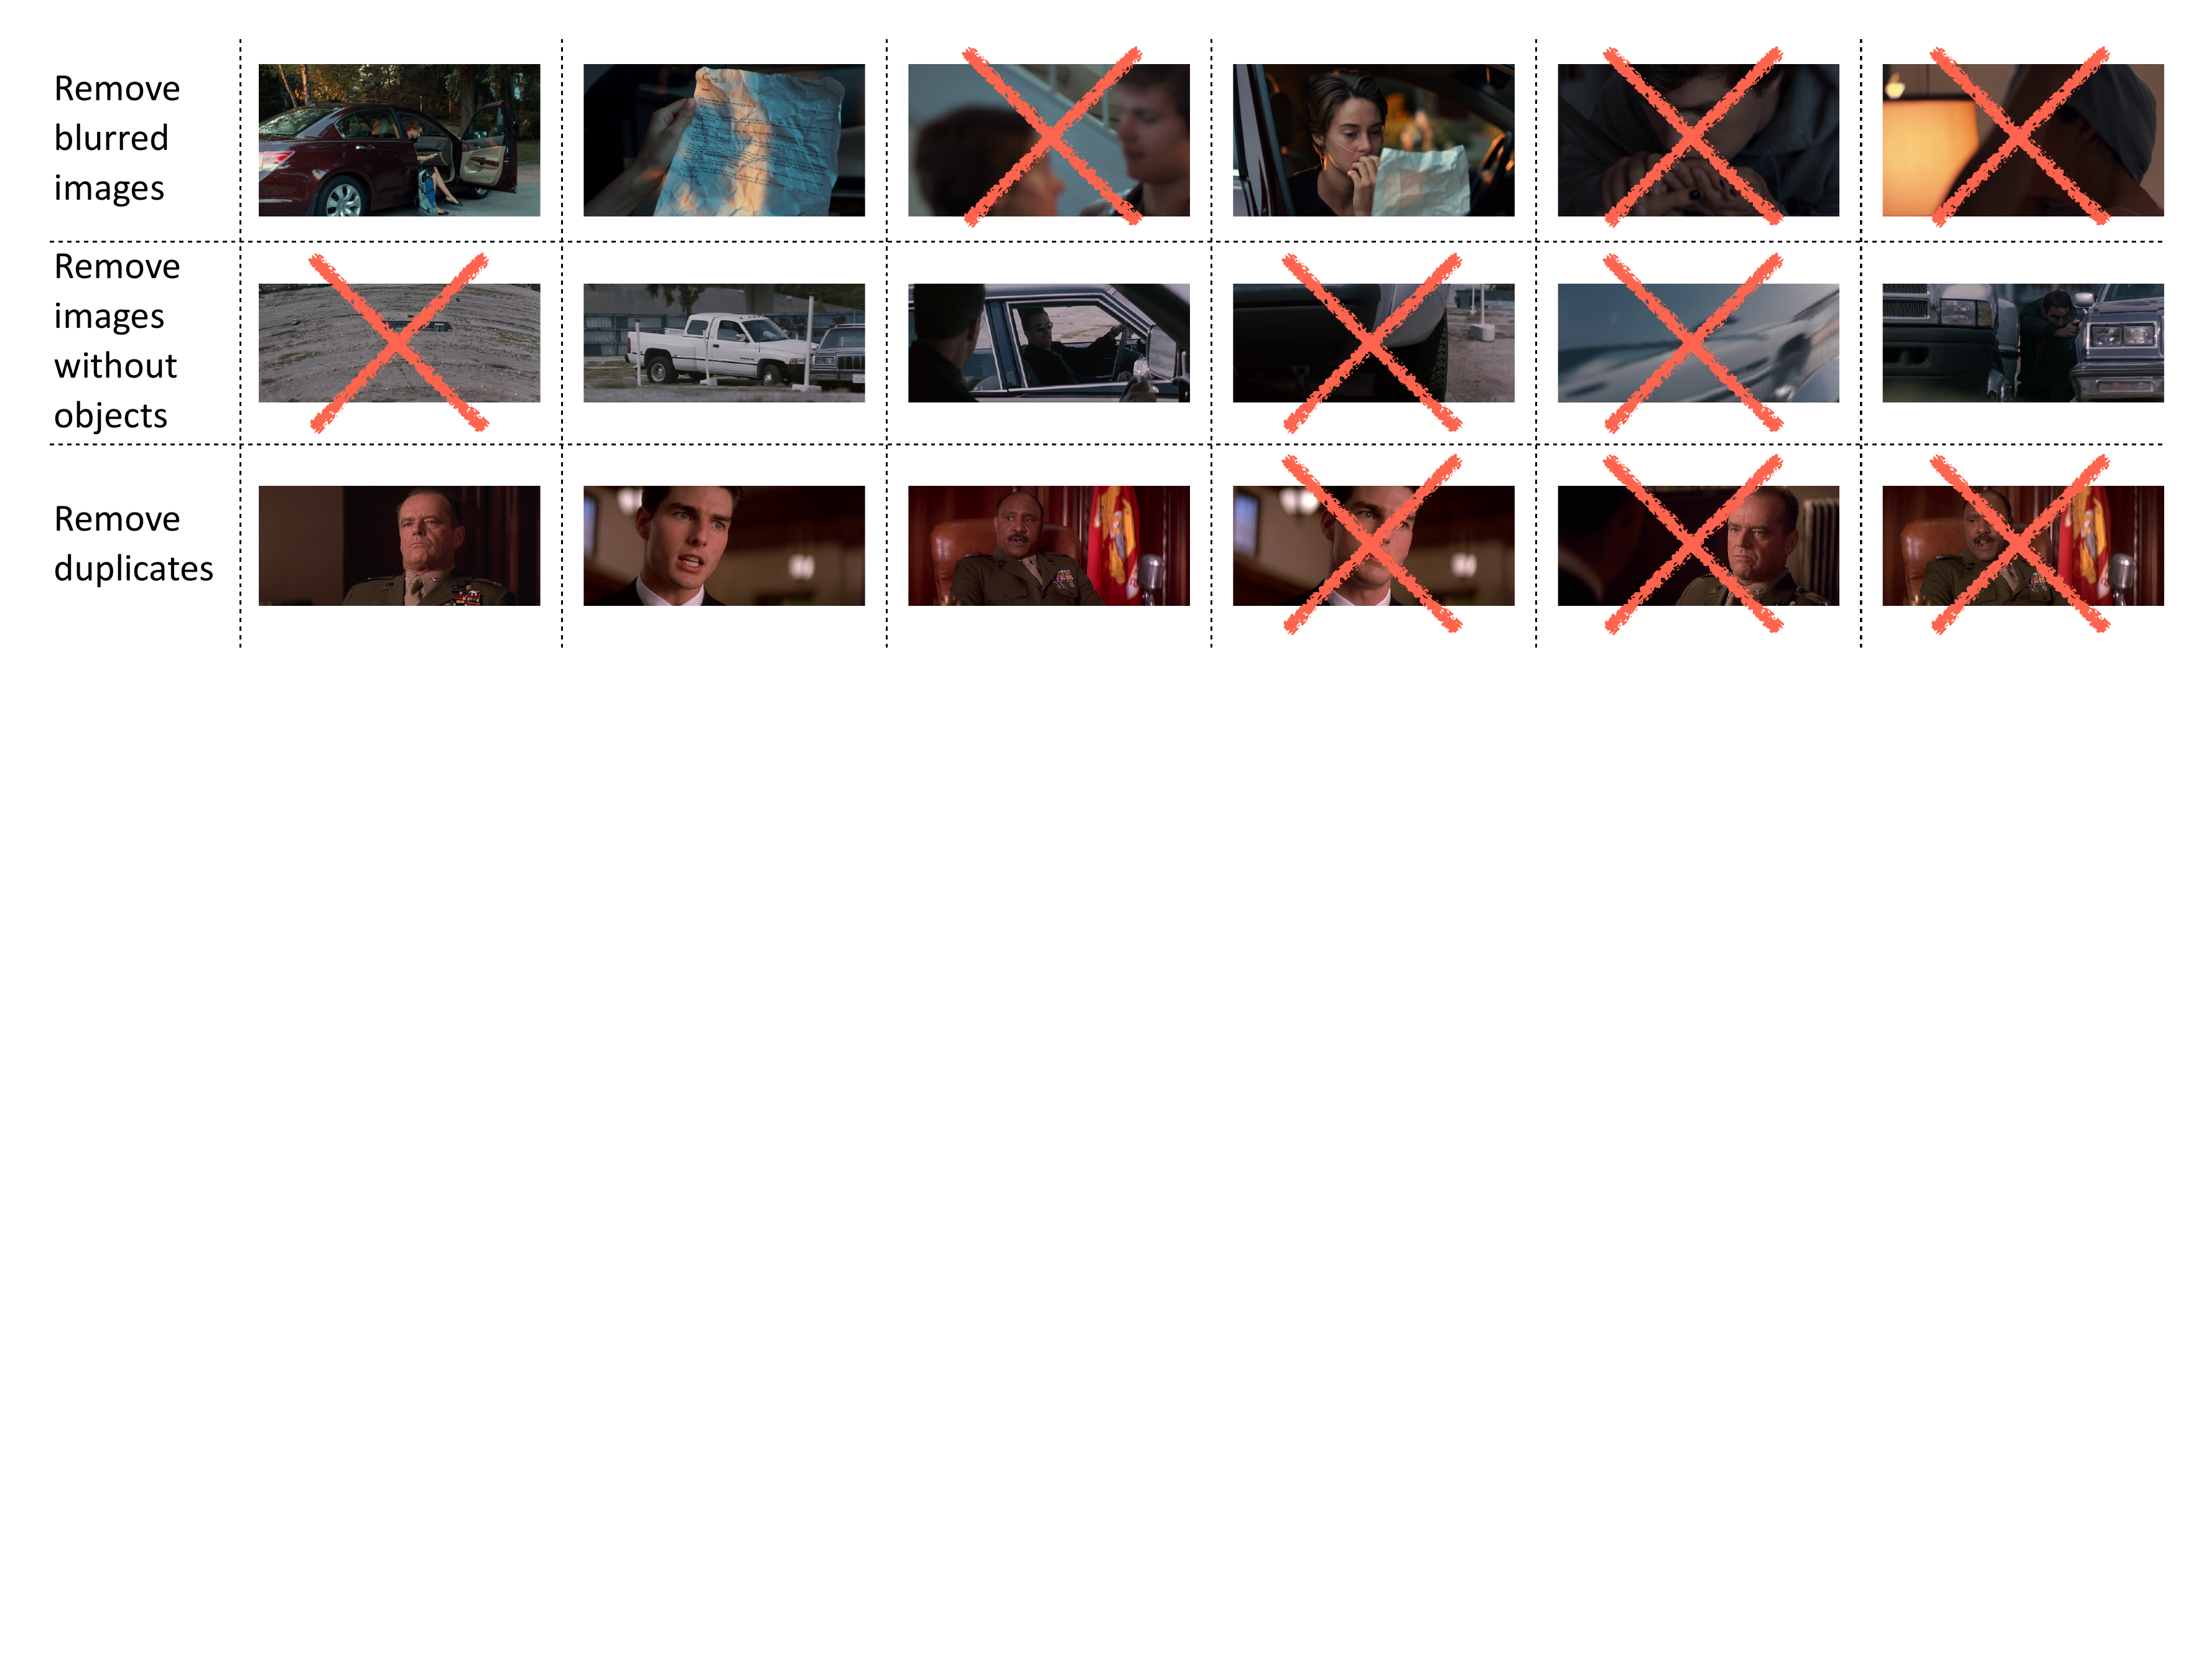}
% \caption{Image filters. }
% \label{fig:img_filter}
% \end{figure*}

% \begin{figure*}[ht]
% \includegraphics[width=0.95\textwidth,trim={0cm 5cm 7cm 0cm},clip]{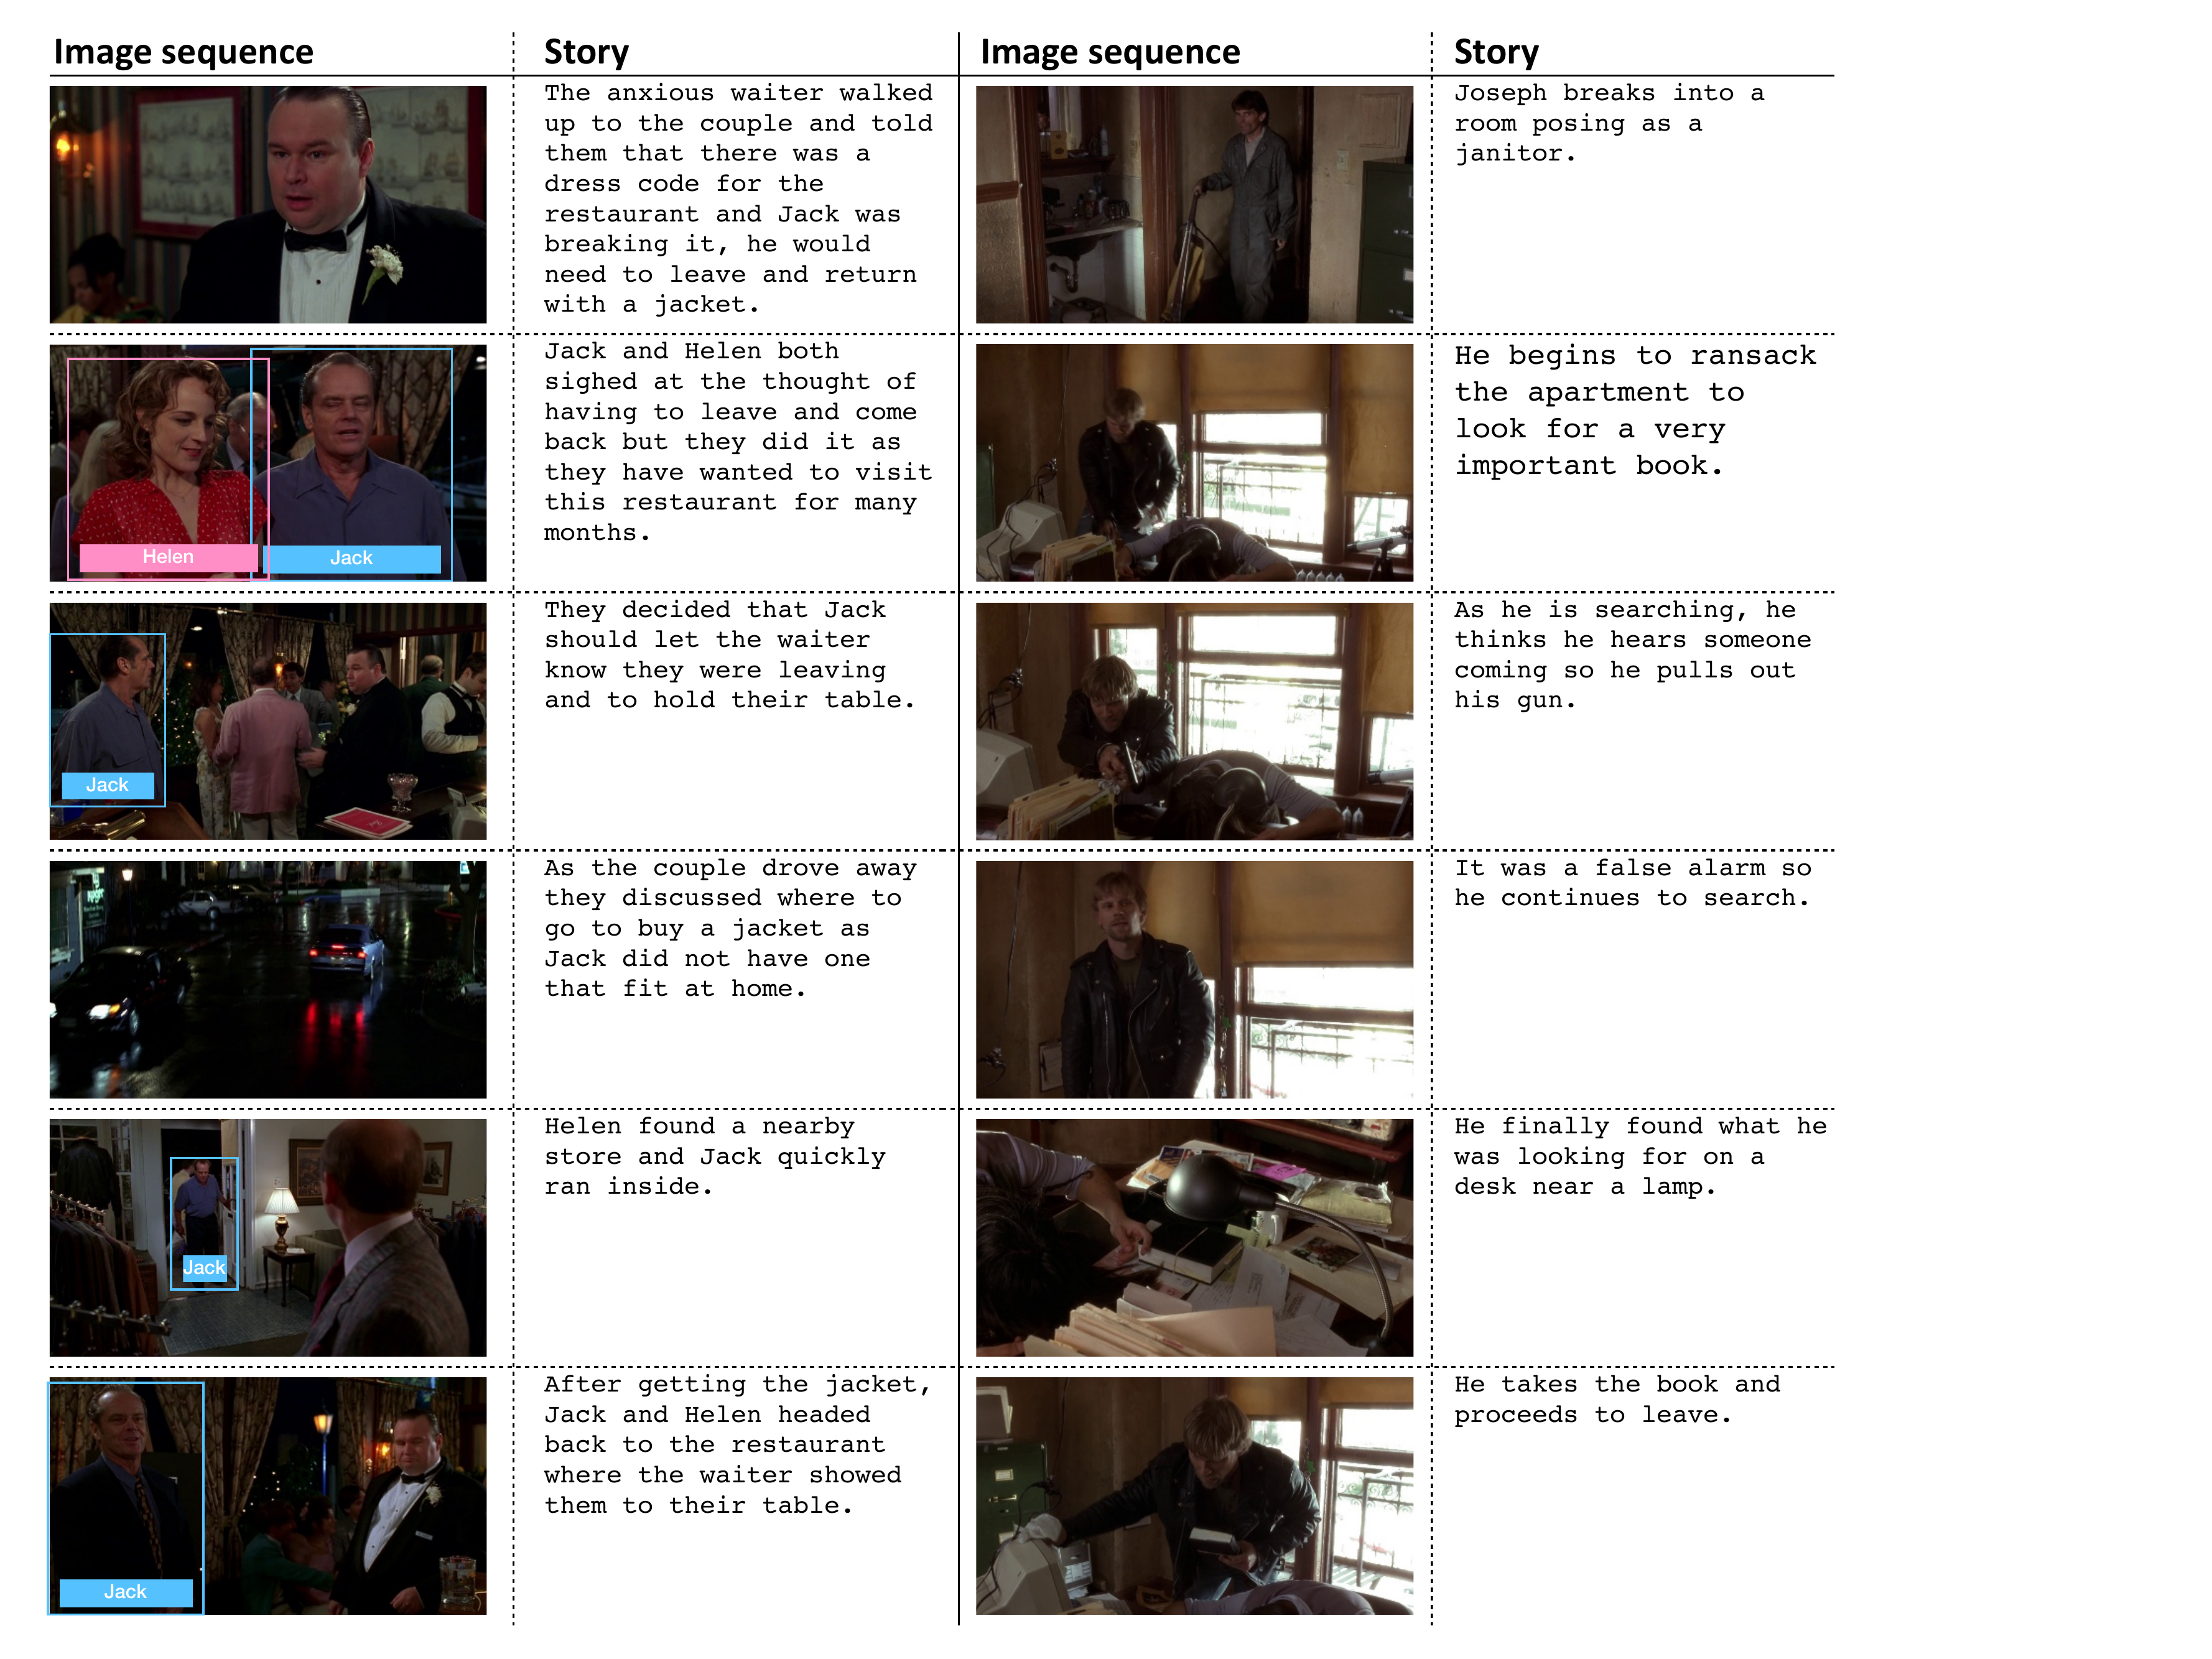}
% \includegraphics[width=0.95\textwidth,trim={0cm 3cm 7cm 0cm},clip]{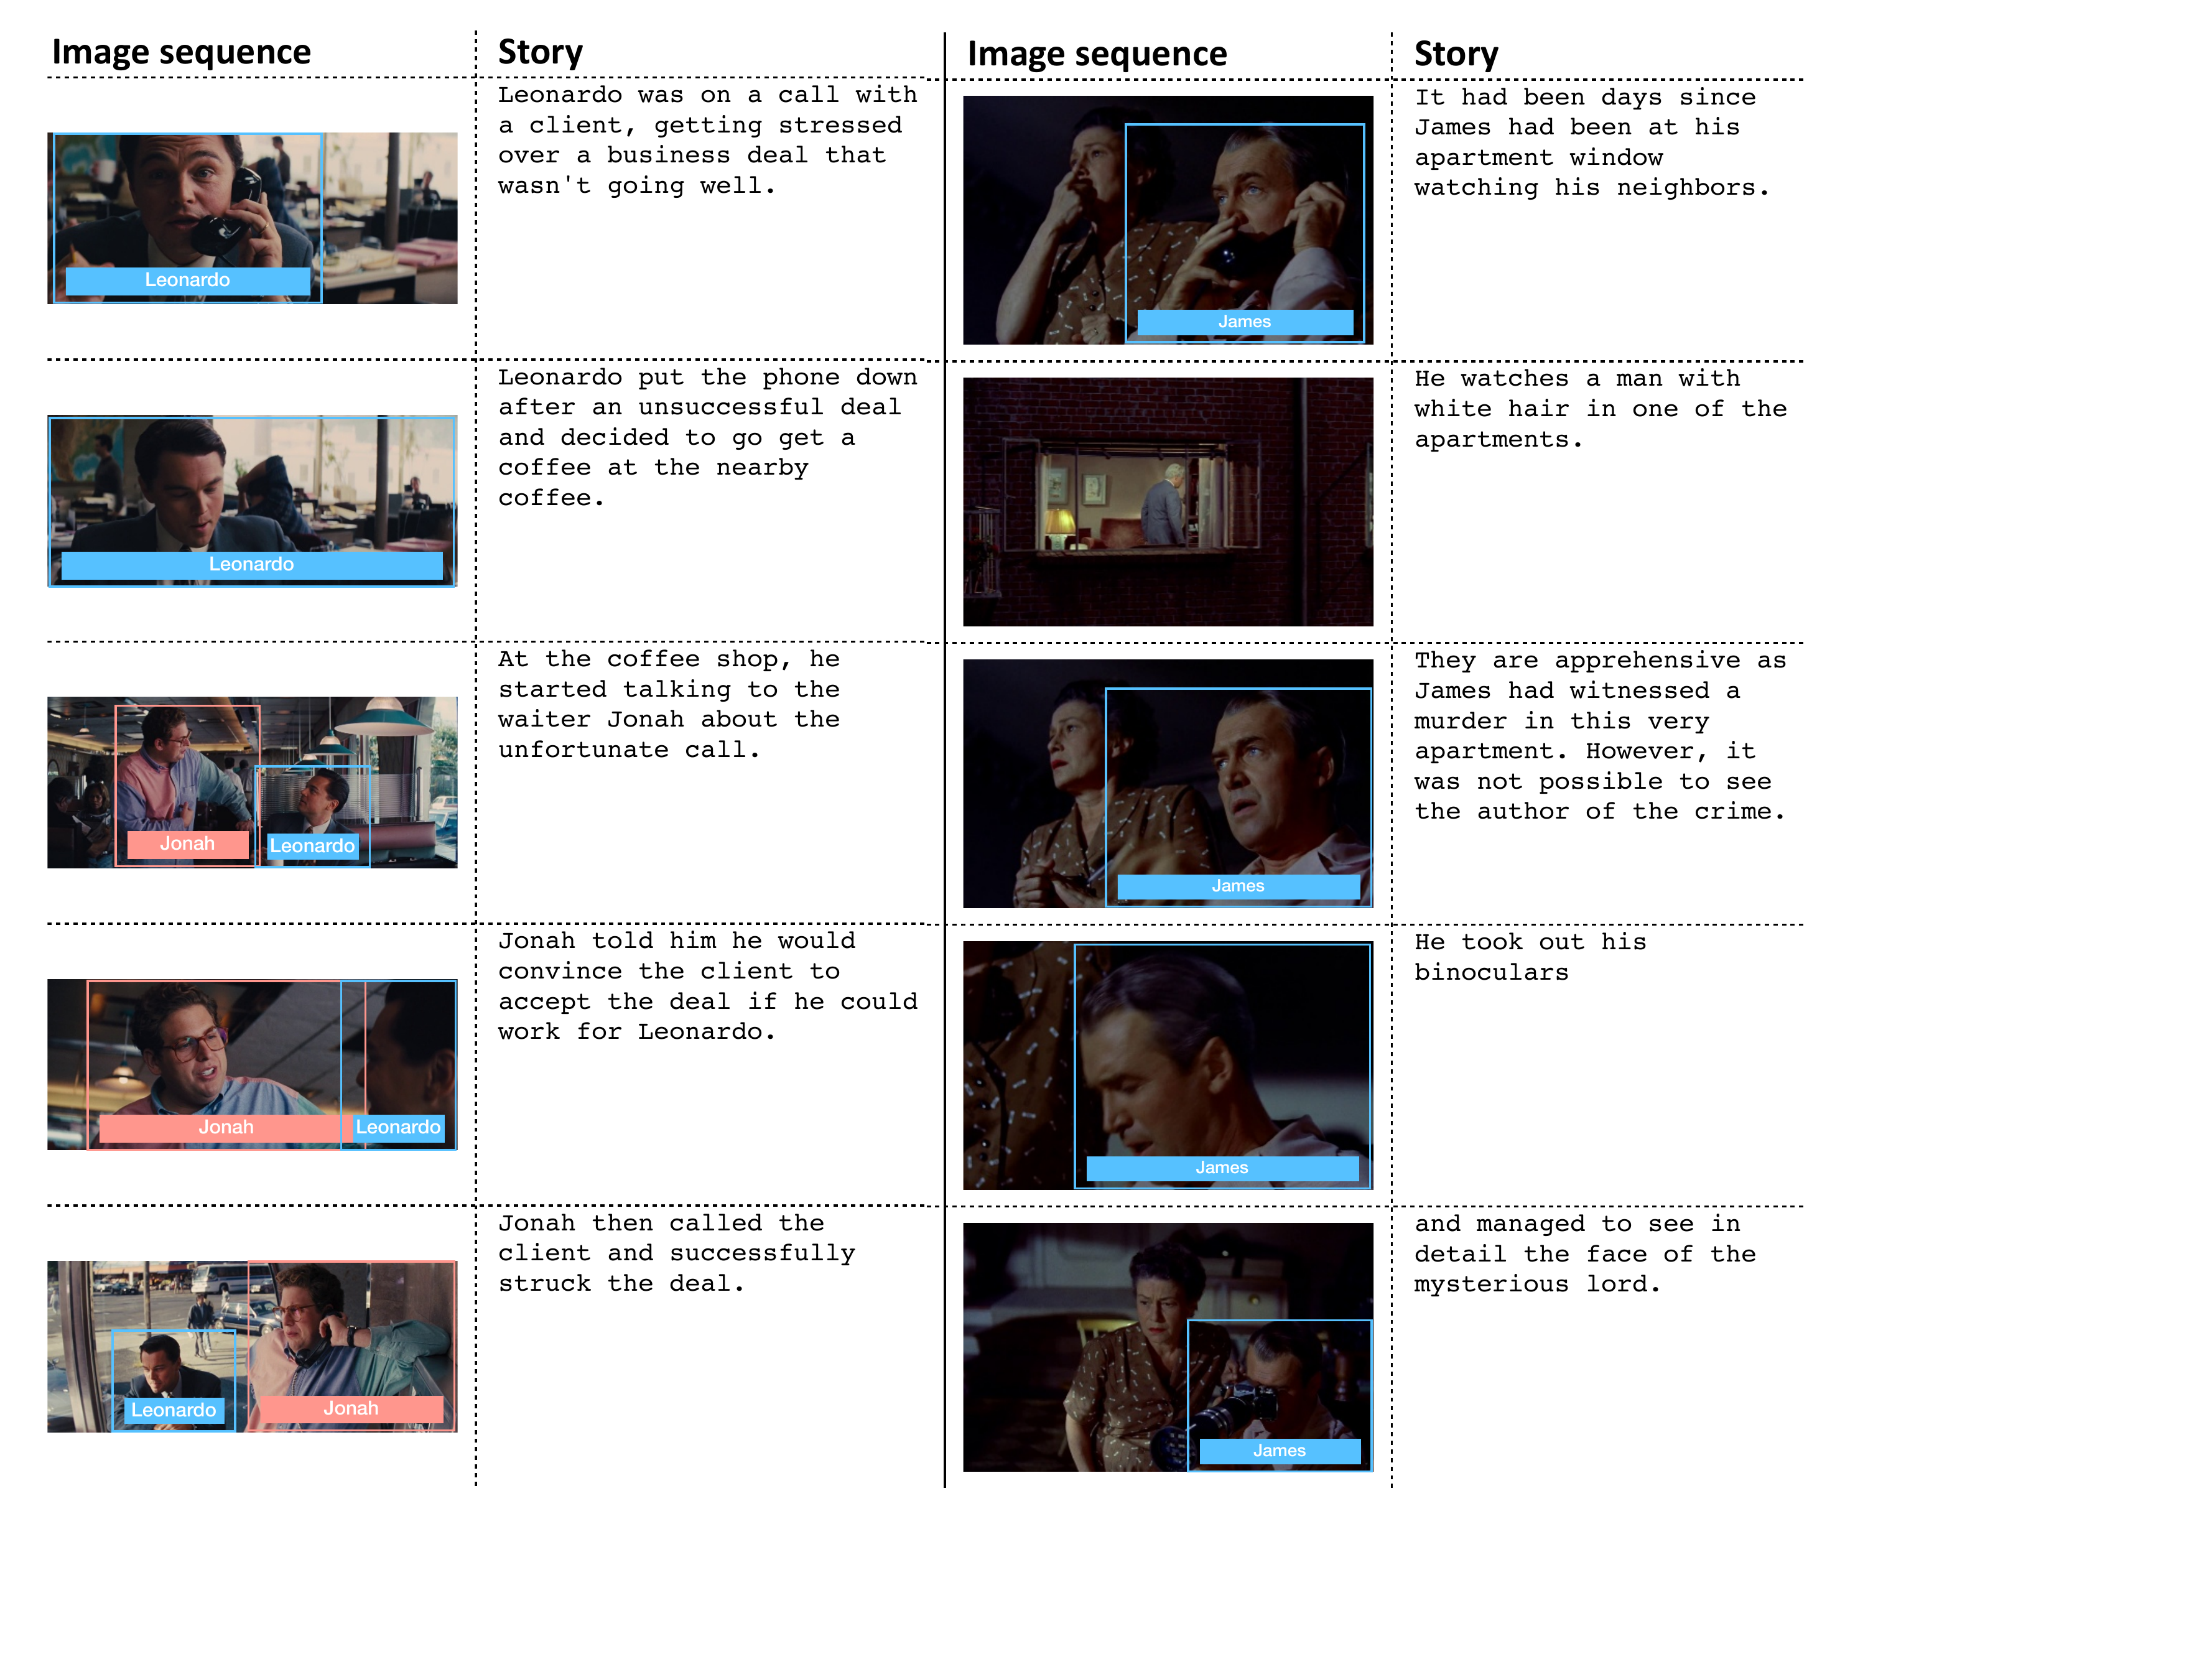}
% \caption{ Worker interface on Amazon Mechanical Turk. }
% \label{fig:example1}
% \end{figure*}

% \begin{figure}[t]
% \includegraphics[width=0.48\textwidth]{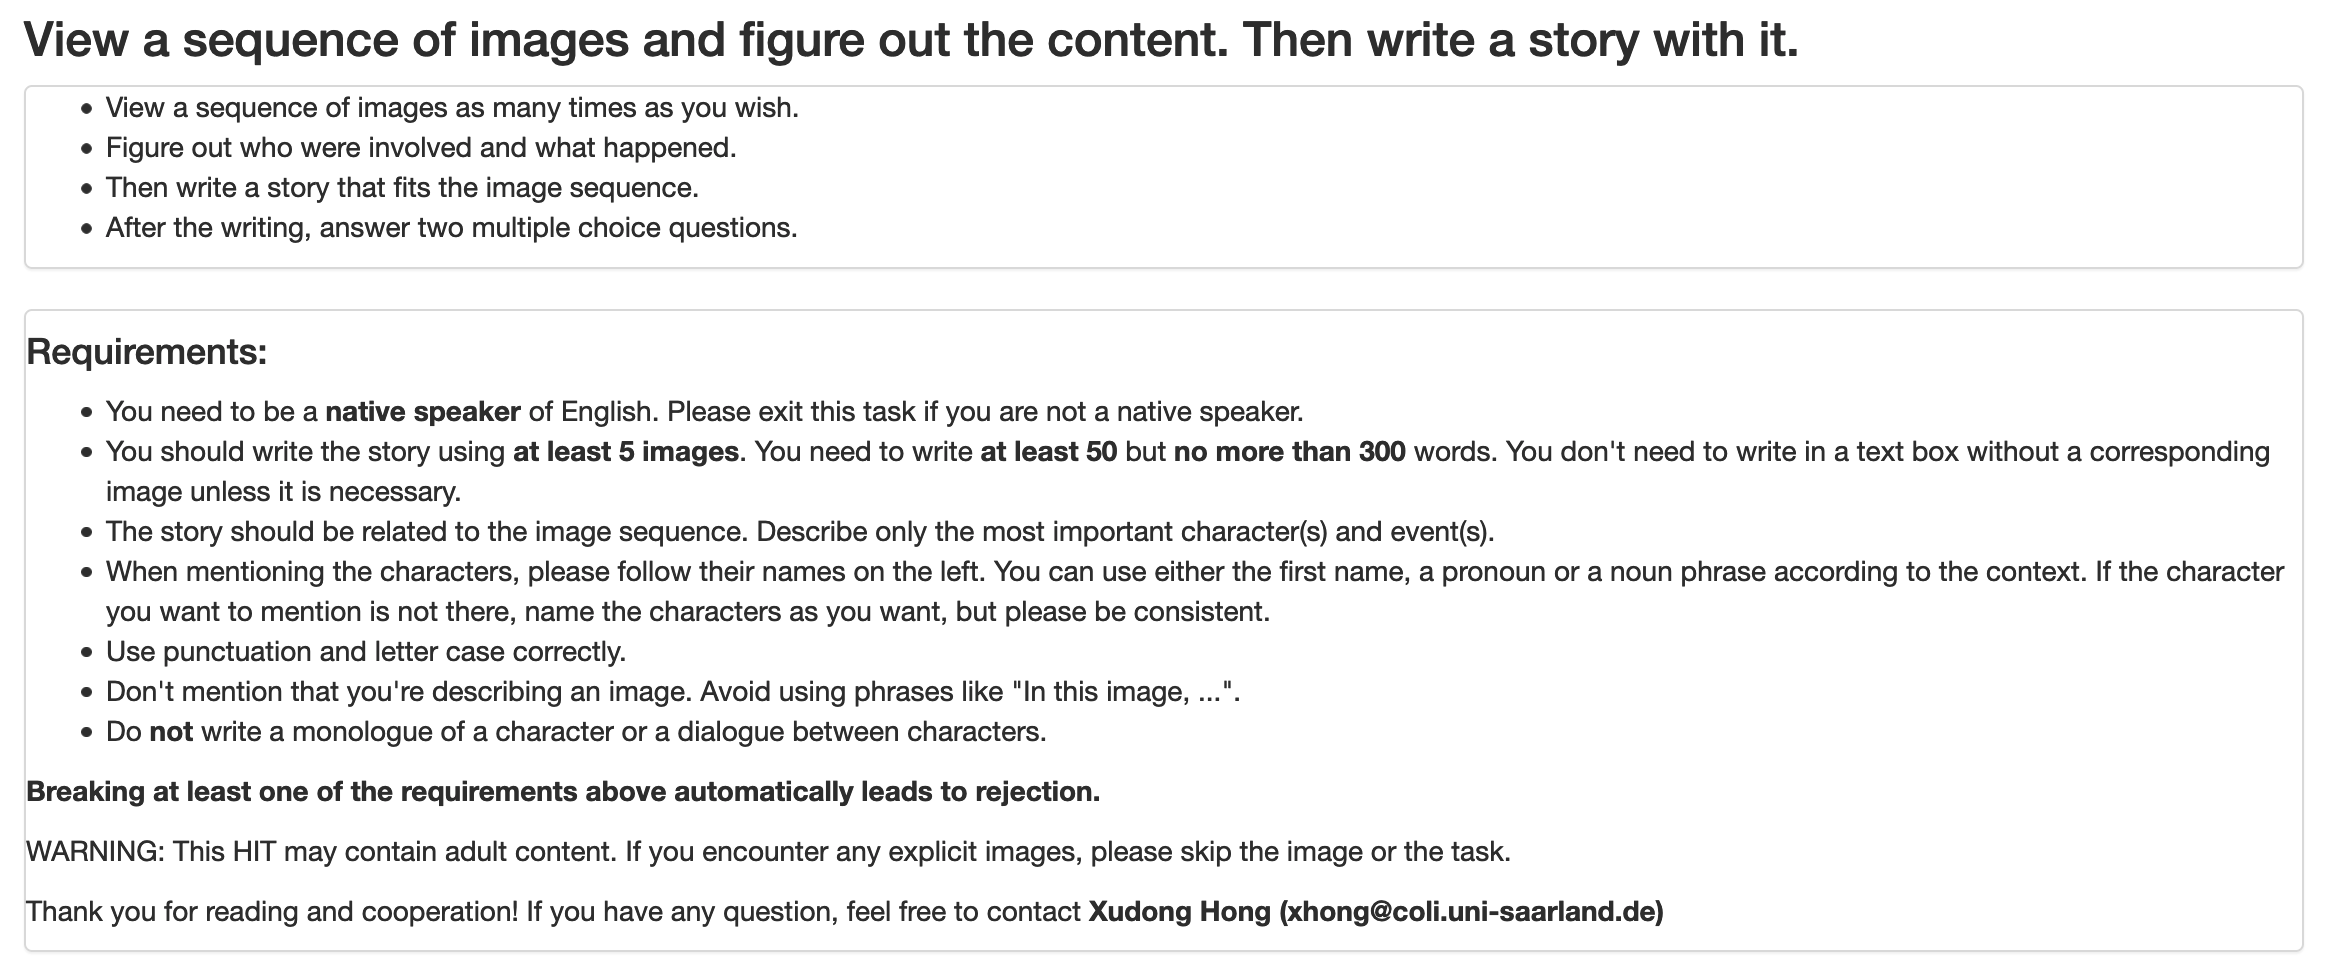}
% \includegraphics[width=0.48\textwidth]{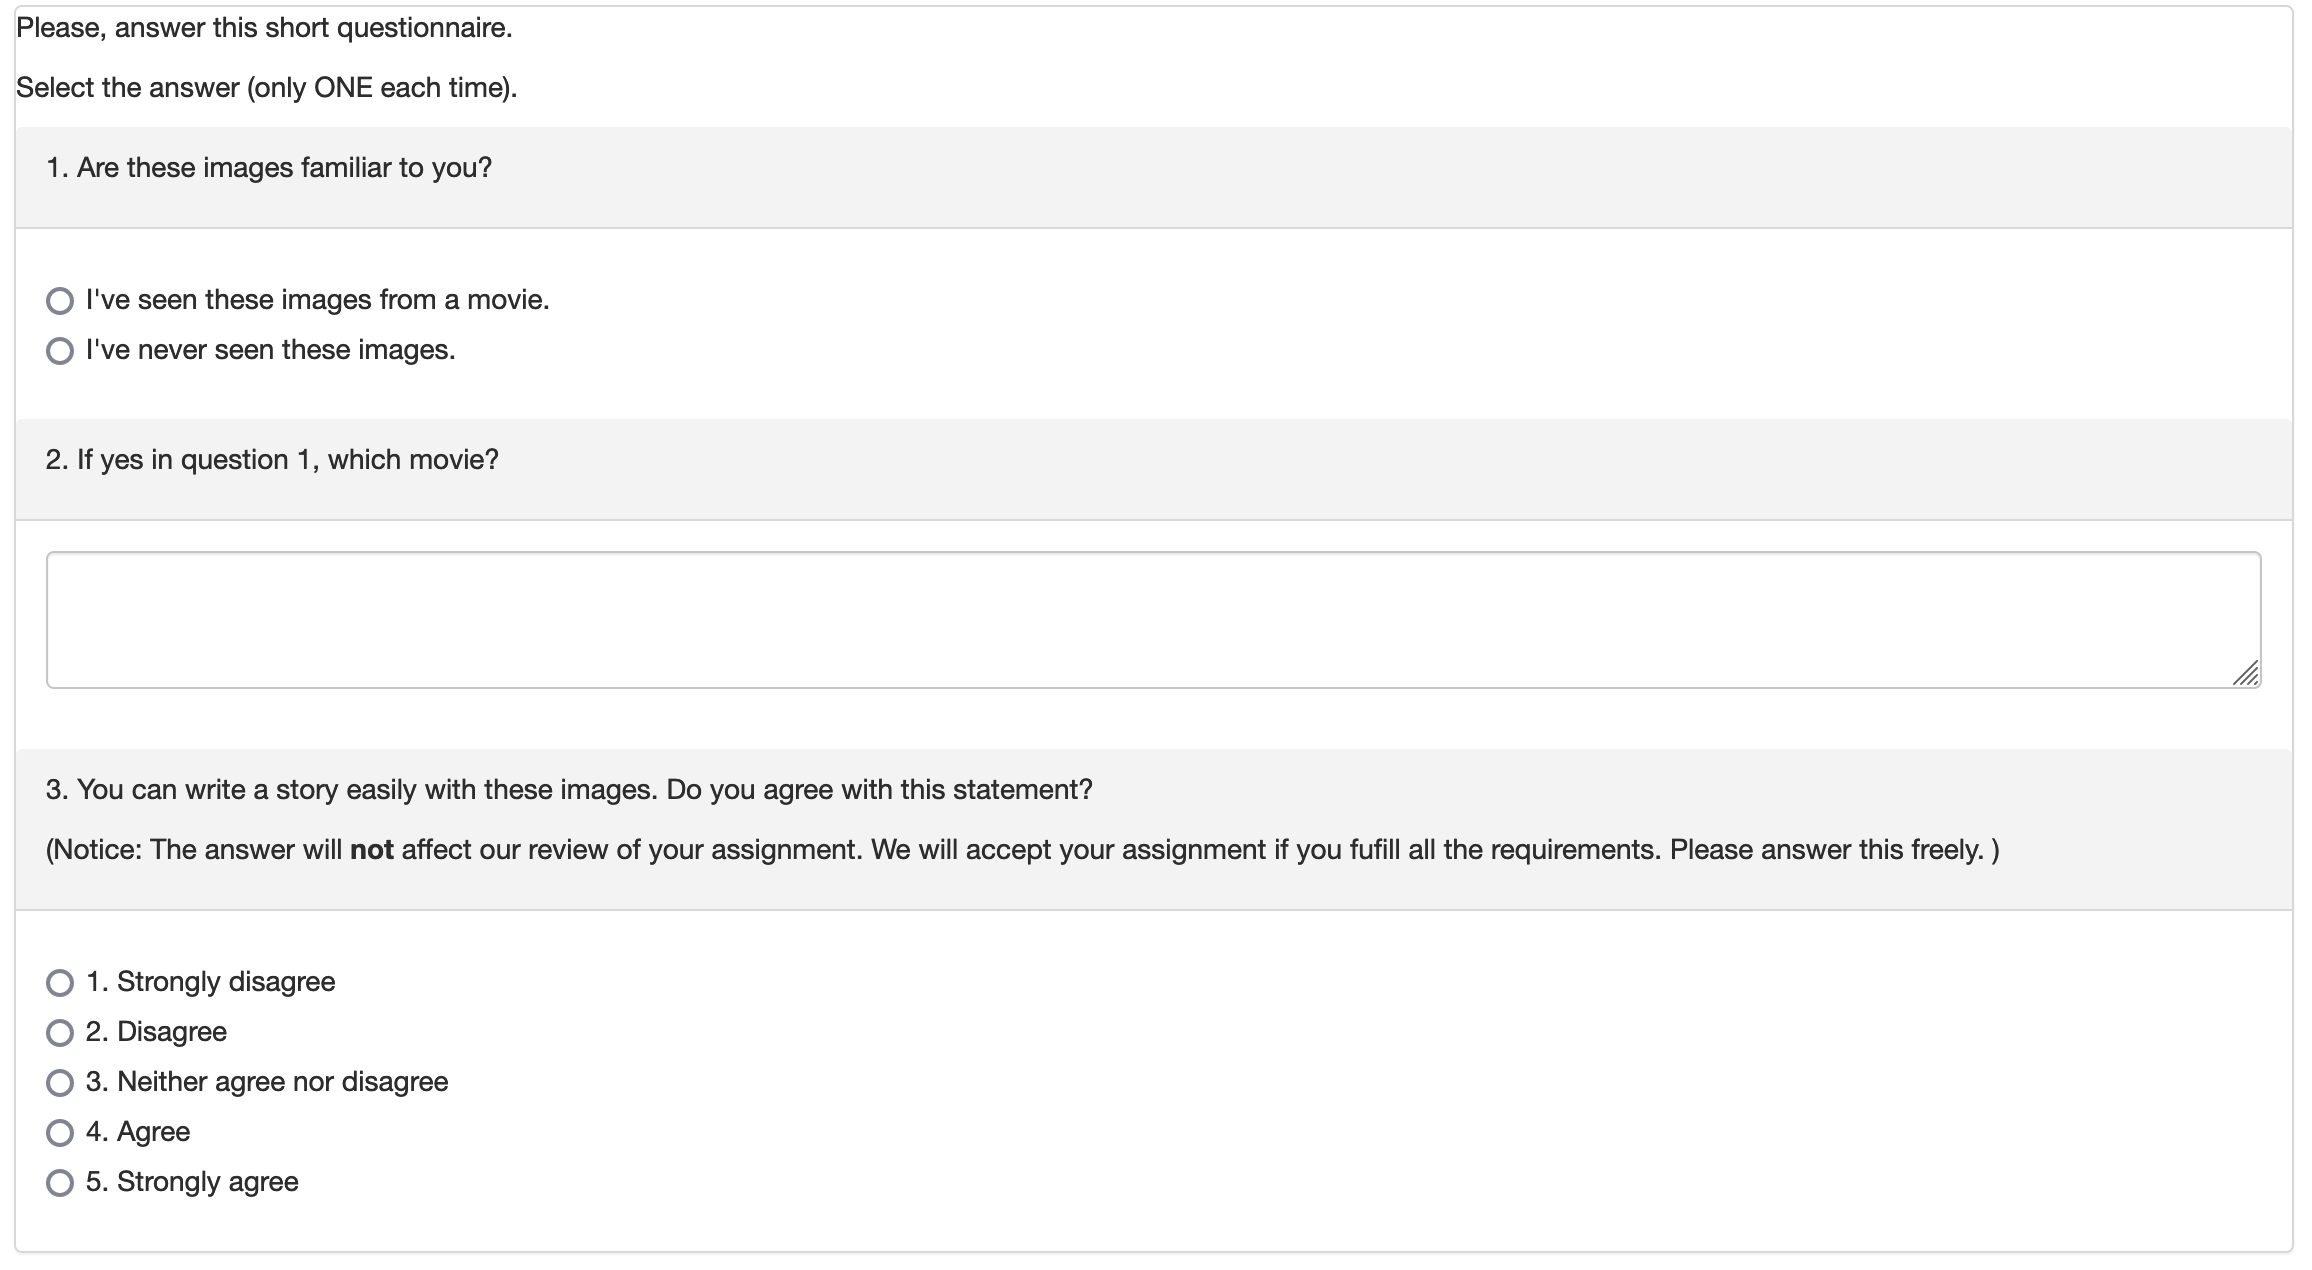}
% \caption{Worker interface on Amazon Mechanical Turk. }
% \label{fig:amt-task}
% \end{figure}

% \begin{figure}[t]

% \caption{Worker interface on Amazon Mechanical Turk. }
% \label{fig:amt-questionnaire}
% \end{figure}

% \begin{figure*}[t]
% \includegraphics[width=0.95\textwidth]{fig/exp1.png}
% \caption{ Task and requirements for worker on Amazon Mechanical Turk. }
% \label{fig:amt-task}
% \end{figure*}

% \begin{figure*}[t]
% \includegraphics[width=0.95\textwidth]{fig/exp3.png}
% \caption{ Questionnaire on Amazon Mechanical Turk. }
% \label{fig:amt-questionnaire}
% \end{figure*}

% XH: specificity
% \subsection{Specificity}

% \subsection{Distribution}
% See Figure \ref{fig:diversity}. 
% \begin{figure*}[t]
%   \centering
% \includegraphics[width=\textwidth]{fig/Adj(without human).png}
% \caption{Frequency verse rank distributions of adjective phrases in generated stories of all models. }
% \label{fig:diversity}
% \end{figure*}
